# Supplementary material for: Graph-Theoretic Formulation of Hamiltonian and Ground-State Sign Structures in Heisenberg Antiferromagnets
Source: arXiv:2602.04943 source file (2026-10-21)
Supplement: Supplementary file 1 [file sm.pdf]

# SUPPLEMENTAL MATERIAL

## Graph–Theoretic Analysis of Phase Optimization Complexity in Variational Wave Functions for Heisenberg Antiferromagnets

Mahmud Ashraf Shamim[1], Md Moshiur Rahman Raj[2], Mohamed Hibat-Allah[3,4] and Paulo T Araujo[1]

[1] *Department of Physics and Astronomy, University of Alabama, Tuscaloosa, 35487, Alabama, USA*
[2] *Department of Physics, University of Rajshahi, P.O. Box 6205, Rajshahi, Bangladesh*
[3] *Department of Applied Mathematics, University of Waterloo, Ontario, Canada N2L 3G1*
[4] *Vector Institute, Toronto, Ontario, M5G 0C6, Canada*

In this Supplemental Material, we (i) provide the derivation of the weighted $XY$ model for the $J_1 - J_2$ Heisenberg antiferromagnet, (ii) proof of the Bipartiteness Inheritance Theorem, (iii) relation between Holonomy and gauge invariance, (iv) Proof of PEC–Bipartiteness Theorem, (v) PEC & ferro-anti ferro system, (vi) proof of Marshall Sign Rule, (vii) construction of $\hat{\eta}_A$ operator, (viii) proof of Sublattice Parity Constraint, (ix) Goemans–Williamson algorithm and bound for the worst cut for HG, (x) Phase Optimization as a QUBO Problem in VMC, (xi) Dirichlet Energy and Graph Laplacian for the Continuous phase optimization, and (xii) Phase optimization for $2 \times 2$ square lattice HAF.

### DERIVATION OF WEIGHTED $XY$ MODEL

Let $G = (V, E)$ be a simple, undirected, connected graph. We interpret this graph as a physical lattice, where quantum spins reside on the vertices and interactions occur along the edges. The set $V = \{i, j, \cdots\}$ is the set of vertices (lattice sites), whose elements we label by $i, j, k, \ldots$, and $E \subset \{\{i, j\} : i, j \in V, i \neq j\}$ is the set of undirected edges between sites. If a geometric embedding of $G$ is specified, we denote its physical dimension by $D$ ($D = 1$ for 1D, $D = 2$ for 2D, $D = 3$ for 3D); however, all definitions below use only the *topological distance* $d_{ij}$ and are independent of $D$. For $i, j \in V$ the topological distance $d_{ij}$ is the shortest path length on $G$, joining $i$ and $j$ (with $d_{ii} = 0$). For each site $i$ we define the $r^{\text{th}}$ neighbor shell as

$$N_r(i) = \{j \in V : d_{ij} = r\}, \qquad r = 1, 2, \cdots \tag{1}$$

Nearest neighbors (NN) are the pairs with $d_{ij} = 1$ and next–nearest neighbors (NNN) are those with $d_{ij} = 2$. Placing spin operators $\hat{\mathbf{S}}_i = (\hat{S}_i^x, \hat{S}_i^y, \hat{S}_i^z)$ on each vertex $i \in V$, for spin-$\frac{1}{2}$ ($\hat{\mathbf{S}}_i = \frac{1}{2}\hat{\boldsymbol{\sigma}}_i$), $J_1 - J_2$ Heisenberg Hamiltonian is

$$\hat{H} = J_1 \sum_{\langle ij \rangle} \hat{\mathbf{S}}_i . \hat{\mathbf{S}}_j + J_2 \sum_{\langle\langle ij \rangle\rangle} \hat{\mathbf{S}}_i . \hat{\mathbf{S}}_j \tag{2}$$

Where the sum $\sum_{\langle ij \rangle}$ runs over *unordered* NN pairs $\{i, j\} \in E$ with $d_{ij} = 1$, and $\sum_{\langle\langle ij \rangle\rangle}$ over unordered NNN pairs with $d_{ij} = 2$. We take $J_1, J_2 > 0$ for antiferromagnetic couplings. Using $S_i^{\pm} := S_i^x \pm i S_i^y$ and $\mathbf{S}_i \cdot \mathbf{S}_j = S_i^z S_j^z + \frac{1}{2}(S_i^+ S_j^- + S_i^- S_j^+)$, we split he Hamiltonian into diagonal and off-diagonal parts $\hat{H} = \hat{H}_{zz} + \hat{H}_{\pm}$ as follows:

$$\hat{H}_{zz} = J_1 \sum_{\langle ij \rangle} \hat{S}_i^z \hat{S}_j^z + J_2 \sum_{\langle\langle ij \rangle\rangle} \hat{S}_i^z \hat{S}_j^z \tag{3}$$

$$\hat{H}_{\pm} = \frac{J_1}{2} \sum_{\langle ij \rangle} \left( \hat{S}_i^+ \hat{S}_j^- + \hat{S}_i^- \hat{S}_j^+ \right) + \frac{J_2}{2} \sum_{\langle\langle ij \rangle\rangle} \left( \hat{S}_i^+ \hat{S}_j^- + \hat{S}_i^- \hat{S}_j^+ \right). \tag{4}$$

In the computational basis, the diagonal part $\hat{H}_{zz}$ counts, for a given $|\sigma\rangle$, the number of antiparallel ("domain-wall") bonds on NN and NNN links. For a single bond $\{ij\}$, the action of the diagonal term is

$$\hat{S}_i^z \hat{S}_j^z |\sigma\rangle = \begin{cases} +\frac{1}{4} |\sigma\rangle, & \text{if spins in } \langle i, j \rangle \text{ parallel} \\ -\frac{1}{4} |\sigma\rangle, & \text{if spins in } \langle i, j \rangle \text{ anti-parallel} \end{cases} \tag{5}$$

Let $a_\sigma^{(1)}$ and $a_\sigma^{(2)}$ denote the numbers of NN and NNN antiparallel bonds in configuration $\sigma$, respectively. Summing over all bonds produces constants proportional to the total bond counts $N_1$ and $N_2$, which merely shift the spectrum uniformly and are therefore discarded. We thus redefine the diagonal part as $\hat{H}_{zz}\,|\sigma\rangle = -\frac{1}{2}\left(J_1 a_\sigma^{(1)} + J_2 a_\sigma^{(2)}\right)|\sigma\rangle$.

The off–diagonal operator $\hat{H}^{\pm}$ connects two configurations only when a single antiparallel pair occurs on an interaction edge. For the $J_1$–$J_2$ system, these edges lie in $E_1$ (NN) or $E_2$ (NNN). Given $\sigma$, choose a bond $\{i,j\} \in E_1 \cup E_2$ with $\sigma_i = -\sigma_j$. Flipping that pair produces a new configuration $\tau$, written $\sigma \to \tau$, and we call this a *Heisenberg flip* (HF). We denote the sets of NN and NNN HFs by $\mathcal{R}_1 = \{(\sigma,\tau) : \sigma \to \tau \text{ via } E_1\}$ and $\mathcal{R}_2 = \{(\sigma,\tau) : \sigma \to \tau \text{ via } E_2\}$, and the corresponding NN and NNN neighbors of $\sigma$ by $\mathcal{N}_1(\sigma) = \{\tau : (\sigma,\tau) \in \mathcal{R}_1\}$ and $\mathcal{N}_2(\sigma) = \{\tau : (\sigma,\tau) \in \mathcal{R}_2\}$. For a given physical graph $G$, we denote its configuration graph by $\Gamma(G) = (\mathcal{V},\mathcal{E})$. Here $\mathcal{V} = \{\uparrow,\downarrow\}^{|V|}$, and $(\sigma,\tau) \in \mathcal{E}$ iff $\tau \in \mathcal{N}_1(\sigma) \cup \mathcal{N}_2(\sigma)$. Hence, the action of $\hat{H}_\pm$ can be expressed explicitly as a weighted sum over all such flippable configurations, yielding

$$\hat{H}_\pm\,|\sigma\rangle = \frac{1}{2}\left(J_1 \sum_{\tau\in\mathcal{N}_1(\sigma)} |\tau\rangle + J_2 \sum_{\tau\in\mathcal{N}_2(\sigma)} |\tau\rangle\right) \tag{6}$$

By combining the diagonal contribution with the off-diagonal action, we obtain the full expression for the Hamiltonian acting on a vertex $|\sigma\rangle$ on the cgraph as

$$\hat{H}\,|\sigma\rangle = \frac{1}{2}\left[-\left(J_1 a_\sigma^{(1)} + J_2 a_\sigma^{(2)}\right)|\sigma\rangle + \left(J_1 \sum_{\tau\in\mathcal{N}_1(\sigma)} |\tau\rangle + J_2 \sum_{\tau\in\mathcal{N}_2(\sigma)} |\tau\rangle\right)\right] \tag{7}$$

We introduce a variational many-body state $|\Psi(\theta)\rangle$, which in the computational basis $\{|\sigma\rangle\}$ takes the form $|\Psi(\theta)\rangle = \sum_\sigma c_\sigma(\theta)\,|\sigma\rangle$. Its quality is measured by the energy expectation value of the Hamiltonian (1), given by the Rayleigh quotient

$$E(\theta) = \frac{\langle\Psi(\theta)|\,\hat{H}\,|\Psi(\theta)\rangle}{\langle\Psi(\theta)|\Psi(\theta)\rangle}. \tag{8}$$

which provides a variational upper bound to the true GS energy. The task of the variational approach is therefore to adjust the parameters $\theta$ so that $E(\theta)$ is minimized. Substituting $|\Psi(\theta)\rangle$ into the energy expression (7), we obtain an explicit functional of the coefficients $c_\sigma(\theta)$. For notational simplicity, we will henceforth write $c_\sigma \equiv c_\sigma(\theta)$, yielding

$$E = \frac{1}{2\sum_\sigma |c_\sigma|^2}\left[-\sum_\sigma \left(J_1 a_\sigma^{(1)} + J_2 a_\sigma^{(2)}\right)|c_\sigma|^2 + \sum_\sigma \left(J_1 \sum_{\tau\in\mathcal{N}_1(\sigma)} c_\sigma^* c_\tau + J_2 \sum_{\tau\in\mathcal{N}_2(\sigma)} c_\sigma^* c_\tau\right)\right] \tag{9}$$

The variational energy $E[\Psi]$ is implicitly understood as a function of the parameters $\theta$. This energy functional in (9) naturally separates into two distinct contributions: a *classical* (diagonal) part and a quantum interference part. The classical contribution, proportional to $a_\sigma$, is guaranteed to be non-positive. Since $a_\sigma$ counts the number of antiferromagnetic bonds and $|c_\sigma|^2$ is manifestly non-negative, their product is necessarily non-negative. With the overall prefactor $-1$, this term always lowers the energy. It therefore acts as a stabilizing background, independent of the detailed structure of the variational state.

By contrast, the *quantum* contribution arises from the off-diagonal bond-flip processes and reflects interference between amplitudes of configurations connected by a single HF. Its sign is not fixed *a priori*, but depends on the relative phases of the coefficients $\{c_\sigma\}$ and the underlying connectivity of the Heisenberg graph. Since all nontrivial effects originate from this interference, it is convenient to single out this part explicitly. We define

$$E_\mathrm{q} = \frac{1}{2\sum_\sigma |c_\sigma|^2}\left[\sum_\sigma \left(J_1 \sum_{\tau\in\mathcal{N}_1(\sigma)} c_\sigma^* c_\tau + J_2 \sum_{\tau\in\mathcal{N}_2(\sigma)} c_\sigma^* c_\tau\right)\right] \tag{10}$$

Minimizing the quantum contribution $E_\mathrm{q}$ for a general complex amplitude $c_\sigma$ is an intrinsically hard problem. Analytically, it is intractable because the interference arises between amplitudes of configurations connected by bond flips, creating a highly entangled structure. A useful simplification is therefore to restrict attention to a sub-class of the problem in which the magnitudes $|c_\sigma|$ are held fixed, while only the phases $\phi_\sigma$ are varied [**?** ]. This isolates

the interference contribution as the sole optimization target. To expose this structure explicitly, we perform a polar decomposition of the amplitudes:

$$c_\sigma = \psi_\sigma e^{i\phi_\sigma}, \qquad \psi_\sigma \geq 0 \tag{11}$$

Because the HG is undirected, each unordered bond between configurations is counted twice in the directed sum. Hence, for $r = 1, 2$, $\sum_\sigma \sum_{\tau \in \mathcal{N}_r(\sigma)} c^*_\sigma c_\tau = \frac{1}{2} \sum_\sigma \sum_{\tau \in \mathcal{N}_r(\sigma)} \Big( c^*_\sigma c_\tau + c^*_\tau c_\sigma \Big)$. Using the polar form, $c^*_\sigma c_\tau + c^*_\tau c_\sigma = \psi_\sigma \psi_\tau \left( e^{i(\phi_\sigma - \phi_\tau)} + e^{-i(\phi_\sigma - \phi_\tau)} \right) = 2\psi_\sigma \psi_\tau \cos(\phi_\sigma - \phi_\tau)$. Inserting this into (9), the quantum contribution becomes

$$E_q = \frac{1}{Z} \sum_{r=1}^{2} J_r \sum_{\{\sigma,\tau\} \in \mathcal{N}_r} \psi_\sigma \psi_\tau \cos\big(\phi_\sigma - \phi_\tau\big). \tag{12}$$

We interpret Eq. (12) as the energy of a *amplitude weighted* XY model on the cgraph. Each many-body basis state $\sigma$ is a vertex; vertices $\sigma$ and $\tau$ are connected if they are related by a single bond flip—nearest–neighbour (NN flips form the set $\mathcal{N}_1(\sigma)$ and next–nearest–neighbour (NNN) flips form $\mathcal{N}_2(\sigma)$. In terms of the amplitude-weighted adjacency matrix of the original text

$$E_q = \sum_{\{\sigma,\tau\} \in \mathcal{E}} W^{\Gamma}_{\sigma\tau} \cos\big(\phi_\sigma - \phi_\tau\big), \tag{13}$$

where $\mathcal{E}$ is the edge set of $\Gamma(G)$ and $W^{\Gamma}_{\sigma\tau}(J_1, J_2) = \frac{1}{Z} \sum_{r=1}^{2} J_r W^{(r)}_{\sigma\tau}$ vanishes unless $\{\sigma, \tau\} \in \mathcal{N}_1 \cup \mathcal{N}_2$.

This formulation makes explicit that the genuinely quantum content of the variational problem resides in the *phase differences along edges of the cgraph*: amplitudes set the interaction strengths (edge weights), whereas phases control constructive or destructive interference through $\cos(\phi_\sigma - \phi_\tau)$. From this perspective, determining the sign structure becomes a problem of phase optimization on the HG.

Unlike the original Marshall proof [1] and standard textbook treatments [2, 3], which establish the sign rule through eigenvalue inequalities and Perron–Frobenius arguments, the present approach isolates these phase degrees of freedom and reformulates the problem as an amplitude-weighted XY model on the HG. This yields a more general and structurally transparent understanding of sign structure, with the MSR recovered as a special case on bipartite graphs.

## PROOF OF BIPARTITENESS INHERITANCE

Fix a physical graph $G = (V, E)$ and a spin-$\frac{1}{2}$ Hilbert space restricted to a fixed $S^z_{\text{tot}}$ sector with

$$N_\uparrow := \#\{i \in V : \sigma_i = \uparrow\} \qquad \text{fixed.} \tag{14}$$

Define the *Hilbert graph* (HG) $\Gamma(G) = (\mathcal{V}, \mathcal{E})$ whose vertices are spin configurations $\sigma$ in this sector, and where $\{\sigma, \tau\} \in \mathcal{E}$ iff $\tau$ is obtained from $\sigma$ by a single nearest-neighbour Heisenberg flip

$$(\uparrow_i \downarrow_j) \leftrightarrow (\downarrow_i \uparrow_j) \qquad \text{on some bond } (i, j) \in E. \tag{15}$$

**Theorem 1** (Bipartiteness inheritance)**.** *If $G = (V_A \cup V_B, E)$ is bipartite, then $\Gamma(G)$ is bipartite.*

*Proof.* Since $G$ is bipartite, every edge $(i, j) \in E$ connects $i \in V_A$ to $j \in V_B$. For any configuration $\sigma$, define the number of up spins on sublattice $A$,

$$N^\uparrow_A(\sigma) := \#\{i \in V_A : \sigma_i = \uparrow\}, \tag{16}$$

and its parity

$$\Pi(\sigma) := N^\uparrow_A(\sigma) \pmod 2 \in \{0, 1\}. \tag{17}$$

Now let $\{\sigma, \tau\} \in \mathcal{E}$ be an HG edge, so that $\tau$ is obtained from $\sigma$ by a Heisenberg flip on some bond $(i, j)$ with $i \in V_A$, $j \in V_B$. By definition of the move, the spins on $(i, j)$ are antiparallel in $\sigma$, hence exactly one site in $V_A$ changes its spin under the flip (namely $i$). Therefore $N^\uparrow_A$ changes by $\pm 1$, implying

$$\Pi(\tau) = \Pi(\sigma) + 1 \qquad (\text{mod } 2). \tag{18}$$

Define a 2-coloring of $\mathcal{V}$ by

$$c(\sigma) := (-1)^{\Pi(\sigma)} \in \{+1, -1\}. \tag{19}$$

Then for every edge $\{\sigma, \tau\} \in \mathcal{E}$ we have $c(\tau) = -c(\sigma)$, so $\Gamma(G)$ is bipartite. □

**Odd-cycle inheritance**

**Theorem 2** (Odd-cycle inheritance)**.** *Assume the sector is nontrivial, i.e.* $1 \le N_\uparrow \le |V| - 1$*. If* $G$ *contains an odd cycle, then* $\Gamma(G)$ *contains an odd cycle. In particular, if* $G$ *contains a triangle, then* $\Gamma(G)$ *contains a triangle. Consequently,* $G$ *non-bipartite implies* $\Gamma(G)$ *non-bipartite (for nontrivial sectors).*

*Proof.* Since $1 \le N_\uparrow \le |V| - 1$, both spin values occur. Fix a triangle $(i, j, k)$ in $G$ and choose a configuration $\sigma$ such that on these three sites

$$(\sigma_i, \sigma_j, \sigma_k) = \begin{cases} (\uparrow, \downarrow, \downarrow), & N_\uparrow \le |V| - 2, \\ (\downarrow, \uparrow, \uparrow), & N_\uparrow = |V| - 1. \end{cases} \tag{20}$$

with all other spins fixed arbitrarily (their values are irrelevant for the existence of the cycle below).
*Triangle case.* If $N_\uparrow \le |V| - 2$, perform a nearest-neighbour Heisenberg flip on $(i, j)$ to obtain $\sigma^{(1)}$ with

$$(\sigma_i^{(1)}, \sigma_j^{(1)}, \sigma_k^{(1)}) = (\downarrow, \uparrow, \downarrow), \tag{21}$$

then flip on $(j, k)$ to obtain $\sigma^{(2)}$ with

$$(\sigma_i^{(2)}, \sigma_j^{(2)}, \sigma_k^{(2)}) = (\downarrow, \downarrow, \uparrow), \tag{22}$$

and finally flip on $(k, i)$, which returns to $\sigma$. Thus

$$\sigma \to \sigma^{(1)} \to \sigma^{(2)} \to \sigma \tag{23}$$

is a 3-cycle in $\Gamma(G)$.
If instead $N_\uparrow = |V| - 1$, start from $(\sigma_i, \sigma_j, \sigma_k) = (\downarrow, \uparrow, \uparrow)$ and flip successively on $(j, k)$, then $(i, k)$, then $(i, j)$:

$$(\downarrow, \uparrow, \uparrow) \xrightarrow{(j,k)} (\downarrow, \downarrow, \downarrow) \quad \text{(not allowed)},$$

so we choose a different admissible sequence: flip successively on $(i, j)$, then $(i, k)$, then $(j, k)$, yielding

$$(\downarrow, \uparrow, \uparrow) \xrightarrow{(i,j)} (\uparrow, \downarrow, \uparrow) \xrightarrow{(i,k)} (\downarrow, \downarrow, \uparrow) \xrightarrow{(j,k)} (\downarrow, \uparrow, \downarrow). \tag{24}$$

Finally flipping on $(i, j)$ returns to $(\downarrow, \uparrow, \uparrow)$, hence again we obtain an odd cycle in $\Gamma(G)$ and $\Gamma(G)$ is non-bipartite.

*General odd cycle.* For a general odd cycle $C = (v_0, v_1, \ldots, v_{2m})$ in $G$, pick a configuration $\sigma$ such that along $C$ we have $\sigma_{v_0} =\uparrow$ and $\sigma_{v_t} =\downarrow$ for $t = 1, \ldots, 2m$, and place the remaining $N_\uparrow - 1$ up spins on vertices in $V \setminus C$ (when $|V \setminus C| \ge N_\uparrow - 1$; otherwise the claim follows by a separate small-graph argument, e.g. when $G = C$). Then successive Heisenberg flips on $(v_t, v_{t+1})$ for $t = 0, \ldots, 2m - 1$ and finally on $(v_{2m}, v_0)$ move this single up spin once around $C$ and return to $\sigma$ after $2m + 1$ steps, producing an odd cycle in $\Gamma(G)$. □

*Token-graph viewpoint.* In a fixed-$N_\uparrow$ sector, $\Gamma(G)$ is isomorphic to the $k$-token graph $F_k(G)$ (with $k = N_\uparrow$), since a Heisenberg flip moves one up spin along a bond to an empty site. In particular, Theorem 1 is consistent with the general bound $\chi(F_k(G)) \le \chi(G)$ for token graphs [4].

## HOLONOMY AND GAUGE INVARIANCE

Let $\Gamma(G) = (\mathcal{V}, \mathcal{E})$ be the HG of the graph $G(V, E)$. A phase field on the $\Gamma(G)$ is a collection $\{\phi_\sigma\}_{\sigma \in \mathcal{V}}$ assigning a phase to each configuration (vertex). For every directed edge $(\sigma, \tau) \in \mathcal{E}$ define

$$g_{\sigma\tau} := e^{i(\phi_\sigma - \phi_\tau)}. \tag{25}$$

For any closed loop $\gamma = (\sigma_0, \sigma_1, \ldots, \sigma_{n-1}, \sigma_n = \sigma_0)$ in $\Gamma(G)$, the *holonomy* of the phase field around $\gamma$ is

$$\mathtt{Hol}_\gamma := \prod_{k=0}^{n-1} g_{\sigma_k \sigma_{k+1}} = e^{i\Delta\phi_\gamma}, \qquad \Delta\phi_\gamma := \sum_{k=0}^{n-1} (\phi_{\sigma_k} - \phi_{\sigma_{k+1}}). \tag{26}$$

We now perform a gauge transformation $\phi_\sigma \mapsto \phi'_\sigma = \phi_\sigma + \alpha_\sigma$ with an arbitrary angle $\alpha_\sigma$ at each vertex. Under this gauge transformation

$$g_{\sigma\tau} \longrightarrow g'_{\sigma\tau} = e^{i(\phi'_\sigma - \phi'_\tau)} = e^{i(\phi_\sigma + \alpha_\sigma - \phi_\tau - \alpha_\tau)} = e^{i\alpha_\sigma} e^{i(\phi_\sigma - \phi_\tau)} e^{-i\alpha_\tau} = e^{i\alpha_\sigma} g_{\sigma\tau} e^{-i\alpha_\tau} = h_\sigma g_{\sigma\tau} h_\tau^{-1} \tag{27}$$

with $h_\sigma = e^{i\alpha_\sigma}$. Therefore, under the gauge transformation $\texttt{Hol}_\gamma$ changes along the loop $\gamma$ as:

$$\texttt{Hol}_\gamma \longrightarrow \texttt{Hol}'_\gamma = \prod_{k=0}^{n-1} g'_{\sigma_k\sigma_{k+1}} = \Big(h_{\sigma_0} g_{\sigma_0\sigma_1} h_{\sigma_1}^{-1}\Big)\Big(h_{\sigma_1} g_{\sigma_1\sigma_2} h_{\sigma_2}^{-1}\Big) \cdots \Big(h_{\sigma_{n-1}} g_{\sigma_{n-1}\sigma_0} h_{\sigma_0}^{-1}\Big) \tag{28}$$

By telescoping $h_{\sigma_1}^{-1}$ at the end of the first factor cancels the $h_{\sigma_1}$ at the start of the second factor and, likewise for $\sigma_2, \cdots, \sigma_{n-1}$. At the very end, because the loop is closed ($\sigma_n = \sigma_0$), the last term cancels with the first. So every internal gauge factor cancels, and we obtain

$$\texttt{Hol}'_\gamma \; = \; \texttt{Hol}_\gamma.$$

Therefore $\texttt{Hol}_\gamma$ is gauge invariant. Using the Holonomy, we now prove the PEC-Bipartiteness theorem.

## PROOF OF PEC–BIPARTITENESS THEOREM

**Theorem 3** (PEC–bipartiteness)**.** *Let $\Gamma(G) = (\mathcal{V}, \mathcal{E})$ be the Hilbert graph (HG) of the physical graph $G(V, E)$. A phase field on $\Gamma(G)$ is a collection $\{\phi_\sigma\}_{\sigma \in \mathcal{V}}$ assigning a phase to each configuration (vertex). For every directed edge $(\sigma, \tau) \in \mathcal{E}$ define*

$$g_{\sigma\tau} := e^{i(\phi_\sigma - \phi_\tau)}. \tag{29}$$

*For an undirected edge $\{\sigma, \tau\}$, we fix an arbitrary orientation when defining $g_{\sigma\tau}$; reversing the orientation replaces $g_{\sigma\tau}$ by its inverse. For any closed loop $\gamma = (\sigma_0, \sigma_1, \ldots, \sigma_{n-1}, \sigma_n = \sigma_0)$ in $\Gamma(G)$, the holonomy of the phase field around $\gamma$ is*

$$\mathit{Hol}_\gamma := \prod_{k=0}^{n-1} g_{\sigma_k\sigma_{k+1}} = e^{i\Delta\phi_\gamma}, \qquad \Delta\phi_\gamma := \sum_{k=0}^{n-1} (\phi_{\sigma_k} - \phi_{\sigma_{k+1}}). \tag{30}$$

*(With this pure-gauge definition, $\mathit{Hol}_\gamma = 1$ for every closed loop $\gamma$ by telescoping.) Then the following are equivalent:*

1. *The HG $\Gamma(G)$ is bipartite.*
2. *There exists a phase assignment satisfying the global $\pi$–edge condition (PEC)*

$$\phi_\sigma - \phi_\tau \equiv \pi \pmod{2\pi} \quad \textit{for all } (\sigma, \tau) \in \mathcal{E}.$$

*Proof.* (1) ⇒ (2): If $\Gamma(G)$ is bipartite, write $\mathcal{V} = \mathcal{A} \cup \mathcal{B}$ with all edges connecting $\mathcal{A}$ to $\mathcal{B}$. Define

$$\phi_\sigma = \begin{cases} 0, & \sigma \in \mathcal{A}, \\ \pi, & \sigma \in \mathcal{B}. \end{cases}$$

Every edge $(\sigma, \tau)$ connects opposite sublattices, so $\phi_\sigma - \phi_\tau \equiv \pi \pmod{2\pi}$; hence the PEC holds on every edge.

(2) ⇒ (1): Assume there is a phase field obeying the PEC on each edge. Let $\gamma = (\sigma_0, \sigma_1, \ldots, \sigma_{n-1}, \sigma_n = \sigma_0)$ be any closed loop in $\Gamma(G)$. Because $\sigma_n = \sigma_0$, the telescoping sum gives

$$\Delta\phi_\gamma = \sum_{k=0}^{n-1} (\phi_{\sigma_k} - \phi_{\sigma_{k+1}}) \equiv 0 \pmod{2\pi}.$$

But the PEC implies each term satisfies $\phi_{\sigma_k} - \phi_{\sigma_{k+1}} \equiv \pi \pmod{2\pi}$, hence

$$\Delta\phi_\gamma \equiv n\pi \pmod{2\pi}.$$

Therefore $n\pi \equiv 0 \pmod{2\pi}$, which forces $n$ to be even. So $\Gamma(G)$ has no odd cycles, and is bipartite. □

The PEC–bipartiteness theorem is the uniform-sign special case of the more general “unfrustrated sign” criterion used in the auxiliary sign-Ising construction [5]. In general, each HG edge $(\sigma, \tau)$ carries an intrinsic $\mathbb{Z}_2$ sign $\eta_{\sigma\tau} = \mathrm{sign}(J_{\sigma\tau})$, and a consistent global sign assignment exists iff every closed loop has trivial $\mathbb{Z}_2$ holonomy (equivalently, loop parity $P(\gamma) = +1$). When $\eta_{\sigma\tau} \equiv +1$ on all active edges, this reduces to requiring $\phi_\sigma - \phi_\tau = \pi$ on every edge, which is possible exactly when $\Gamma(G)$ is bipartite.

## PEC & FERRO-ANTI FERRO SYSTEM

We now analyze the mixed-coupling case of Eq. (10): antiferromagnetic NN ($J_1 > 0$) and ferromagnetic NNN ($J_2 < 0$). From Eq. (10), the AFM–FM system is obtained by the replacement $J_2 \to -|J_2|$, so the NNN interference enters with a negative prefactor:

$$E_q(\theta) = \frac{1}{2\sum_\sigma |c_\sigma|^2} \sum_\sigma \left( J_1 \sum_{\tau \in \mathcal{N}_1(\sigma)} c_\sigma^* c_\tau - |J_2| \sum_{\tau \in \mathcal{N}_2(\sigma)} c_\sigma^* c_\tau \right). \tag{31}$$

Using $c_\sigma = \psi_\sigma e^{i\phi_\sigma}$ gives

$$E_q(\theta) = \frac{1}{2\sum_\sigma \psi_\sigma^2} \left[ J_1 \sum_\sigma \sum_{\tau \in \mathcal{N}_1(\sigma)} \psi_\sigma \psi_\tau \cos(\phi_\sigma - \phi_\tau) - |J_2| \sum_\sigma \sum_{\tau \in \mathcal{N}_2(\sigma)} \psi_\sigma \psi_\tau \cos(\phi_\sigma - \phi_\tau) \right]. \tag{32}$$

From Eq. (32), the NN sum has a positive prefactor $J_1 > 0$ and is minimized by $\Delta\phi = \pi$ on every NN edge; The NNN sum has a negative prefactor $-|J_2|$ and is minimized by $\Delta\phi = 0$ on every NNN edge. Up to a global $U(1)$ phase, this phase assignment uniquely minimizes each edge contribution for fixed amplitudes $\{\psi_\sigma\}$.

On any bipartite lattice set $\phi = 0$ on sublattice $A$ and $\phi = \pi$ on sublattice $B$. Then NN ($A - -B$) edges have $\Delta\phi = \pi$ and NNN ($A - -A$ or $B - -B$) edges have $\Delta\phi = 0$; all physical loops have trivial holonomy. Thus, the mixed AFM–FM model is sign-unfrustrated: PEC holds on NN edges (with a 0-edge condition on NNN).

## PROOF OF MARSHALL SIGN RULE

Let the physical lattice be bipartite $G = A \cup B$. For a configuration $\sigma$, define

$$p(\sigma) := N_A^{\uparrow}(\sigma) \in \mathbb{Z}$$

the number of up-spins on sublattice $A$ in $\sigma$. Consider any edge flip $\sigma \leftrightarrow \tau$ in the configuration graph (i.e $\tau \in \mathcal{N}(\sigma)$). This edge corresponds to flipping an antiparallel nearest-neighbor bond $\langle i, j \rangle$ with $i \in A$ and $j \in B$. Exactly one of the two cases holds:

- $i \in A$ is $\uparrow$ and $j \in B$ is $\downarrow$: the flip makes $i \downarrow$, so $N_A^{\uparrow}$ decrease by 1.
- $i \in A$ is $\downarrow$ and $j \in B$ is $\uparrow$: the flip makes $i \uparrow$, so $N_A^{\uparrow}$ increase by 1.

Hence, along every edge,

$$p(\tau) = p(\sigma) \pm 1 \quad \Longrightarrow \quad p(\tau) - p(\sigma) \equiv 1 \pmod 2 \tag{33}$$

Therefore, choose the phase

$$\phi_\sigma = \pi p(\sigma), \qquad p(\sigma) = N_A^{\uparrow}(\sigma) \tag{34}$$

Then for every $\tau \in \mathcal{N}(\sigma)$, $\phi_\sigma - \phi_\tau \equiv \pi \pmod{2\pi}$. So the PEC is satisfied globally. Equivalently, the wavefunction coefficients can be written as

$$c_\sigma = e^{i\pi N_A^{\uparrow}(\sigma)} \psi_\sigma = (-1)^{N_A^{\uparrow}} \psi_\sigma. \tag{35}$$

Therefore, the phase become $(-1)^{N_A^{\uparrow}}$ is fixed and *independent* of the variational parameters, making the total wavefunction real up to a global sign.

$$c_\sigma(\theta) = (-1)^{N_A^{\uparrow}(\sigma)} \psi_\sigma(\theta) \tag{36}$$

Inserting it back into the variational wavefunction above gives

$$|\Psi(\theta)\rangle = \sum_\sigma (-1)^{N_A^{\uparrow}(\sigma)} \psi_\sigma(\theta) |\sigma\rangle, \qquad \psi_\sigma(\theta) > 0 \tag{37}$$

This reproduces the Marshall sign structure for the NN HAF. While the original proof of Marshall [1] relies on proof by contradiction, the present derivation identifies the sign structure directly as a consequence of PEC and HG bipartiteness.

We now define a diagonal unitary operator $\hat{\eta}_A$ known as Lieb-Mattis (LM) parity operator [6] that makes the wavefunction positive and rotates the eigenproblem. Let $A$ be a sublattice and set

$$\hat{\eta}_A \left|\sigma\right\rangle = (-1)^{N_A^{\uparrow}(\sigma)} \left|\sigma\right\rangle, \qquad \hat{\eta}_A^{\dagger} = \hat{\eta}_A = \hat{\eta}_A^{-1} \tag{38}$$

Acting with $\hat{\eta}_A$ removes the parity sign and yields a sign-free wavefunction:

$$\left|\Psi'(\theta)\right\rangle = \hat{\eta}_A \left|\Psi(\theta)\right\rangle = \sum_{\sigma} \psi_{\sigma}(\theta) \left|\sigma\right\rangle, \qquad \psi_{\sigma}(\theta) \geq 0 \tag{39}$$

Applying this operator to the Schrödinger equation $\hat{H}_{\text{nn}} \left|\Psi\right\rangle = E \left|\Psi\right\rangle$ of NN Heisenberg antiferromagnet Hamiltonian $\hat{H}$ gives

$$\left(\hat{\eta}_A \hat{H}_{\text{nn}} \hat{\eta}_A\right) \left(\hat{\eta}_A \left|\Psi(\sigma)\right\rangle\right) = E \hat{\eta}_A \left|\Psi(\theta)\right\rangle \tag{40}$$

i.e.

$$\hat{H}'_{\text{nn}} \left|\Psi'(\theta)\right\rangle = E \left|\Psi'(\theta)\right\rangle, \qquad \hat{H}'_{\text{nn}} = \hat{\eta}_A \hat{H}_{\text{nn}} \hat{\eta}_A \tag{41}$$

The LM operator $\hat{\eta}_A$ implements the PEC (Marshall) phase globally, removing all signs in the wavefunction and rendering $\psi_{\sigma}(\theta) \geq 0$. Consequently, the transformed Hamiltonian $\hat{H}'_{\text{nn}} = \hat{\eta}_A \hat{H}_{\text{nn}} \hat{\eta}_A$ has non-positive off-diagonal matrix elements in the computational basis, a property known as *stoquasticity*. We now explicitly construct $\hat{\eta}_A$.

## LM PARITY OPERATOR: DEFINITION AND PROPERTIES

Let $G$ be a bipartite graph with sublattices $A$ and $B$. The number operator counting the up-spins on sublattice $A$ is defined as

$$\hat{N}_A^{\uparrow} = \sum_{i \in A} \frac{1}{2} \left(\mathbb{1} + \hat{\sigma}_i^z\right), \tag{42}$$

where $\hat{\sigma}_i^z$ has eigenvalues $\pm 1$. The Lieb Mattis (*LM parity operator*) is then defined by

$$\hat{\eta}_A = (-1)^{\hat{N}_A}. \tag{43}$$

We introduce the spin-up projection operator for site $i \in A$,

$$\hat{\Pi}_i^{\uparrow} = \frac{1}{2} \left(\mathbb{1} + \hat{\sigma}_i^z\right), \tag{44}$$

which satisfies the following properties:

1. **Idempotence:**

$$\left(\hat{\Pi}_i^{\uparrow}\right)^2 = \hat{\Pi}_i^{\uparrow} \tag{45}$$

2. **Completeness and Orthogonality:** Defining $\hat{\Pi}_i^{\downarrow} = \frac{1}{2}(\mathbb{1} - \hat{\sigma}_i^z)$, we have

$$\hat{\Pi}_i^{\uparrow} + \hat{\Pi}_i^{\downarrow} = \mathbb{1}, \qquad \hat{\Pi}_i^{\uparrow} \hat{\Pi}_i^{\downarrow} = 0. \tag{46}$$

3. **Action on the $\hat{\sigma}^z$ Basis:** For the local spin states,

$$\hat{\Pi}_i^{\uparrow} \left|\uparrow\right\rangle_i = \left|\uparrow\right\rangle_i, \qquad \hat{\Pi}_i^{\uparrow} \left|\downarrow\right\rangle_i = 0. \tag{47}$$

Using these projectors, the LM parity operator can be written as

$$\hat{\eta} = (-1)^{\sum_{i\in A} \hat{\Pi}_i^{\uparrow}}. \tag{48}$$

We now compute the action of $(-1)^{\hat{\Pi}^{\uparrow}}$ on a single site:

$$\begin{aligned}(-1)^{\hat{\Pi}^{\uparrow}} &= \exp\Big(\pi i\, \hat{\Pi}^{\uparrow}\Big) = \mathbb{1} + \sum_{n=1}^{\infty} \frac{(\pi i)^n}{n!} (\hat{\Pi}^{\uparrow})^n \\ &= \mathbb{1} + \big(e^{\pi i} - 1\big)\hat{\Pi}^{\uparrow} = \mathbb{1} - 2\hat{\Pi}^{\uparrow} = -\hat{\sigma}^z. \end{aligned} \tag{49}$$

This operator identity also follows directly from the spectral calculus, since the function $f(x) = (-1)^x$ is Borel measurable on the spectrum $\{0, 1\}$ of $\hat{\Pi}^{\uparrow} = (1 + \hat{\sigma}^z)/2$. Therefore, for the full sublattice $A$,

$$\hat{\eta}_A = (-1)^{\sum_{i\in A} \hat{\Pi}_i^{\uparrow}} = (-1)^{n_A} \prod_{i\in A} \hat{\sigma}_i^z, \tag{50}$$

where $n_A$ is the number of sites in sublattice $A$. For even $n_A$, the overall phase is trivial and the operator reduces to

$$\hat{\eta}_A = \prod_{i\in A} \hat{\sigma}_i^z. \tag{51}$$

## Commutation with Total Magnetization

Because $\hat{\eta}$ and $S^z_{\text{tot}} = \sum_i \sigma_i^z/2$ are both diagonal in the $\sigma^z$ basis,

$$\big[\tilde{H},\, S^z_{\text{tot}}\big] = \big[\hat{\eta}_A\, H\, \hat{\eta}_A^{-1},\, S^z_{\text{tot}}\big] \tag{52}$$

$$\begin{aligned} &= \hat{\eta}_A\, [H,\, S^z_{\text{tot}}]\, \hat{\eta}_A^{-1} + [\hat{\eta}_A,\, S^z_{\text{tot}}]\, H\, \hat{\eta}_A^{-1} + \hat{\eta}_A\, H\, [\hat{\eta}_A^{-1},\, S^z_{\text{tot}}] \\ &= 0 \end{aligned} \tag{53}$$

Since, $[H, S^z_{\text{tot}}] = [\hat{\eta}, S^z_{\text{tot}}] = 0$. Thus, $\tilde{H}$ commutes with $S^z_{\text{tot}}$ and preserves each magnetization sector. Equivalently, one can choose a basis of simultaneous eigenstates of $\tilde{H}$ and $S^z_{\text{tot}}$, so $\tilde{H}$ decomposes into independent blocks labeled by the total-$S^z$ quantum number.

## PROOF OF SUBLATTICE PARITY CONSTRAINT

**Theorem 4** (Sublattice Parity Constraint on Bipartite Graphs). *Let $G = (V, E)$ be a finite, connected, bipartite graph with vertex partition $V = A \cup B$ and $|A| = n_A$, $|B| = n_B$ denote the numbers of sites in the sublattices $A$ and $B$ respectively. For a spin-$\frac{1}{2}$ system on $G$, define*

$$\hat{\eta}_A := \prod_{i\in A} \hat{\sigma}_i^z, \qquad \hat{\eta}_B := \prod_{j\in B} \hat{\sigma}_j^z.$$

*Let $n_\downarrow$ denote the number of down spins in the state that is fixed in any $S^z_{\text{tot}}$ sector. Then the following identities hold algebraically:*

*(i) For any bipartite graph (even or odd number of vertices),*

$$\hat{\eta}_A \hat{\eta}_B = \prod_{i\in V} \hat{\sigma}_i^z = (-1)^{n_\downarrow}\, \mathbb{1}.$$

*(ii) Suppose in addition that $G$ has an even number of vertices $N = |V| = 2n_A$ so that $|A| = |B| = n_A$, and that there exists a unitary graph automorphism $\hat{S}$ which exchanges the two sublattices,*

$$\hat{S}(A) = B, \qquad \hat{S}(B) = A.$$

*Working in the zero-magnetization sector* $S^z_{\rm tot} = 0$*, we have* $n_\downarrow = N/2 = n_A$*. By statement (i), which implies*

$$\hat\eta_B = (-1)^{n_\downarrow}\hat\eta_A.$$

*Since* $\hat S$ *maps* $A$ *to* $B$*, it follows that*

$$S\hat\eta_A S^{-1} = \hat\eta_B = (-1)^{n_A}\hat\eta_A.$$

*For any eigenstate* $|\psi\rangle$ *of* $\hat S$*,* $\hat S|\psi\rangle = e^{i\kappa}|\psi\rangle$*, this implies*

$$\big[1-(-1)^{n_A}\big]\langle\hat\eta_A\rangle_\psi = 0.$$

*In particular:*

- *If* $N = 4L$*, then* $n_A$ *is even and no constraint is imposed on* $\langle\hat\eta_A\rangle_\psi$*.*
- *If* $N = 4L+2$*, then* $n_A$ *is odd and therefore*

$$\langle\hat\eta_A\rangle_\psi = 0. \tag{54}$$

*(iii) If* $G$ *has an odd number of vertices* $N = 2n_A + 1$*, then* $|A| \neq |B|$*, and no graph automorphism can exchange the two sublattices. In this case statement (i) still holds, but no analogue of the constraint in (ii) is possible:* $\langle\hat\eta_A\rangle_\psi$ *and* $\langle\hat\eta_B\rangle_\psi$ *are not forced to vanish by symmetry.*

*Proof.* (i) Fix an $S^z$–basis configuration $|\sigma\rangle = |\sigma_1,\ldots,\sigma_{|V|}\rangle$ with eigenvalues $\hat\sigma^z_i|\sigma\rangle = s_i|\sigma\rangle$, $s_i = \pm1$. Let $n_\downarrow$ be the number of down spins in this configuration, i.e. the number of sites with $s_i = -1$. Then

$$\hat\eta_A\hat\eta_B|\sigma\rangle = \Big(\prod_{i\in A} s_i\Big)\Big(\prod_{j\in B} s_j\Big)|\sigma\rangle = \Big(\prod_{k\in V} s_k\Big)|\sigma\rangle = (-1)^{n_\downarrow}|\sigma\rangle.$$

Therefore, within any fixed $S^z_{\rm tot}$ sector (where $n_\downarrow$ is fixed),

$$\hat\eta_A\hat\eta_B = (-1)^{n_\downarrow}\,\mathbb{1}.$$

Since $\hat\eta_A^2 = \hat\eta_B^2 = \mathbb{1}$, this may be rewritten as

$$\hat\eta_B = (-1)^{n_\downarrow}\hat\eta_A,$$

showing that $\hat\eta_A$ and $\hat\eta_B$ are not independent.

(ii) Now assume $N = |V|$ is even and the bipartition has equal sizes $|A| = |B| = n_A$ so that $N = 2n_A$, and work in the zero–magnetization sector $S^z_{\rm tot} = 0$. Then $n_\downarrow = N/2$ and by (i)

$$\hat\eta_A\hat\eta_B = \prod_{i\in V}\hat\sigma^z_i = (-1)^{N/2}\mathbb{1} = (-1)^{n_A}\mathbb{1},$$

which implies

$$\hat\eta_B = (-1)^{n_A}\hat\eta_A. \tag{55}$$

Let $\hat S$ be a unitary graph automorphism that exchanges the two sublattices, $\hat S(A) = B$ and $\hat S(B) = A$. The induced permutation of vertices satisfies $\hat S\hat\sigma^z_i\hat S^{-1} = \hat\sigma^z_{\pi(i)}$ for some bijection $\pi : V \to V$. Thus

$$\hat S\hat\eta_A\hat S^{-1} = \hat S\Big(\prod_{i\in A}\hat\sigma^z_i\Big)\hat S^{-1} = \prod_{i\in A}\hat\sigma^z_{\pi(i)} = \prod_{j\in B}\hat\sigma^z_j = \hat\eta_B.$$

Combining this with (55) gives

$$\hat S\hat\eta_A\hat S^{-1} = \hat\eta_B = (-1)^{n_A}\hat\eta_A.$$

Now let $|\psi\rangle$ be an eigenstate of $\hat S$, $\hat S|\psi\rangle = e^{i\kappa}|\psi\rangle$. Then

$$\begin{aligned}\langle\hat\eta_A\rangle_\psi &= \langle\psi|\hat\eta_A|\psi\rangle = \langle\psi|\hat S^{-1}\big(\hat S\hat\eta_A\hat S^{-1}\big)\hat S|\psi\rangle\\ &= \langle\psi|\hat S^{-1}\big((-1)^{n_A}\hat\eta_A\big)\hat S|\psi\rangle\\ &= (-1)^{n_A}\langle\psi|\hat S^{-1}\hat\eta_A\hat S|\psi\rangle = (-1)^{n_A}\langle\psi|\hat\eta_A|\psi\rangle = (-1)^{n_A}\langle\hat\eta_A\rangle_\psi.\end{aligned}$$

Hence

$$\big[1-(-1)^{n_A}\big]\langle\hat{\eta}_A\rangle_\psi = 0. \tag{56}$$

If $N=4L$, then $n_A$ is even and no constraint on $\langle\hat{\eta}_A\rangle_\psi$ follows. If $N=4L+2$ then $n_A$ is odd and we obtain

$$\langle\hat{\eta}_A\rangle_\psi = 0, \tag{57}$$

as claimed.

(iii) Finally, suppose $G$ has an odd number of vertices $N=2n_A+1$. Then in any bipartition $V=A\cup B$ one has $|A|\neq|B|$. If there existed a graph automorphism $S$ with $\hat{S}(A)=B$ and $\hat{S}(B)=A$, then by bijectivity we would have $|B|=|\hat{S}(A)|=|A|$, which contradicts $|A|\neq|B|$. Thus, no symmetry can exchange the two sublattices when $N$ is odd, so the argument in (ii) cannot be applied. Statement (i) continues to hold, but $\langle\hat{\eta}_A\rangle_\psi$ and $\langle\hat{\eta}_B\rangle_\psi$ are not forced to vanish by symmetry. □

## GOEMANS–WILLIAMSON ALGORITHM

In this section, we review the Goemans–Williamson (GW) algorithm [7], a standard approximation method for the MaxCut problem that combines a semidefinite programming (SDP) [8] relaxation with a randomized rounding scheme.

Let $\Gamma(G)=(\mathcal{V},\mathcal{E})$ be an undirected HG with nonnegative edge weights $W_{\sigma\tau}\geq 0$. A *cut* is specified by the Ising variables $s_i\in\{+1,-1\}$ on vertices, where an edge is cut if $s_i\neq s_j$. The weighted cut value is

$$\mathsf{Cut}(s)=\sum_{(\sigma,\tau)\in\mathcal{E}} W_{\sigma\tau}\left(\frac{1-s_\sigma s_\tau}{2}\right). \tag{58}$$

Thus, MaxCut is equivalent to minimizing an antiferromagnetic Ising energy $\sum_{(\sigma,\tau)} W_{\sigma\tau}s_\sigma s_\tau$ or, equivalently, maximizing $\mathsf{Cut}(s)$.

GW algorithm replaces the Ising spins $s_\sigma\in\{\pm1\}$ with unit vectors $\mathbf{v}_\sigma\in\mathbb{R}^n$ for some $n\leq|V|$. Using $\mathbf{v}_\sigma.\mathbf{v}_\tau$ as a continuous proxy for $s_\sigma s_\tau$, it relax MaxCut to

$$\max_{\{\mathbf{v}_\sigma\}}\sum_{(\sigma,\tau)\in\mathcal{E}} W_{\sigma\tau}\left(\frac{1-\mathbf{v}_\sigma\cdot\mathbf{v}_\tau}{2}\right)\quad \text{s.t.}\quad \|\mathbf{v}_\sigma\|=1\ \ \forall\sigma. \tag{59}$$

Equivalently, define the Gram matrix $X\in\mathbb{R}^{|V|\times|V|}$ by $X_{\sigma\tau}=\mathbf{v}_\sigma\cdot\mathbf{v}_\tau$, so that $X=V^\top V$, where $V\in\mathbb{R}^{n\times|V|}$ is the matrix whose $\sigma$-th column is $\mathbf{v}_\sigma$. By construction, $X\succeq 0$ and $\mathrm{diag}(X)=1$, and the relaxed MaxCut becomes the SDP

$$\max_{X\succeq 0}\sum_{(\sigma,\tau)\in\mathcal{E}} W_{\sigma\tau}\left(\frac{1-X_{\sigma\tau}}{2}\right)\quad \text{s.t.}\quad X_{\sigma\sigma}=1\ \ \forall\sigma. \tag{60}$$

This convex program can be solved in polynomial time to obtain an optimal solution $X^\star$, which can be factorized (e.g., via Cholesky or eigen decomposition) as $X^\star=V^\top V$, yielding a set of unit vectors $\{\mathbf{v}_\sigma\}$.

The SDP solution gives a set of unit vectors $\{v_\sigma\}$ instead of the Ising spins $\pm1$. GW converts them into a discrete cut using a random hyperplane through the origin: (i) Sample a random direction $r$ uniformly from the unit sphere. (ii) Assign a spin by the sign of the projection:

$$s_\sigma=\mathrm{sign}(r.\mathbf{v}_\sigma) \tag{61}$$

Geometrically, the hyperplane perpendicular to $r$ separates the vectors into two half-spaces; vertices landing on opposite sides form the cut. For an edge $(\sigma,\tau)$, if the angle between $v_\sigma$ and $v_\tau$ is $\theta_{\sigma\tau}\in[0,\pi]$, then the probability that the hyperplane separates them is $\Pr[s_\sigma\neq s_\tau]=\frac{\theta_{\sigma\tau}}{\pi}$. Hence, the expected rounded cut value is

$$\mathbb{E}[\mathsf{Cut}(s)]=\sum_{(\sigma,\tau)\in\mathcal{E}} W_{\sigma\tau}\frac{\theta_{\sigma\tau}}{\pi} \tag{62}$$

The SDP objective contributes per edge is $\frac{1}{2}(1 - v_\sigma v_\tau) = \frac{1}{2}(1 - \cos\theta_{\sigma\tau})$. Goemans and Williamson showed that, for all $\theta_{\sigma\tau} \in [0, \pi]$,

$$\frac{\theta_{\sigma\tau}/\pi}{(1 - \cos\theta_{\sigma\tau})/2} \geq \alpha_{\mathrm{GW}}, \tag{63}$$

where $\alpha_{\mathrm{GW}} \approx 0.87856$. Therefore, the random-hyperplane rounding produces a cut whose expected value is at least $\mathbb{E}[\mathsf{Cut}(s)] \geq \alpha_{\mathrm{GW}}.\mathtt{opt}$, where $\mathtt{opt}$ is the true $\mathsf{MaxCut}$ optimum. Repeating the rounding multiple times and taking the best cut boosts the probability of achieving a near-expected outcome.

## PHASE OPTIMIZATION AS A MAX-CUT INSTANCE IN VARIATIONAL MONTE CARLO

We write the variational neural quantum state in amplitude–phase form

$$\Psi_\theta(\sigma) = \psi_\theta(\sigma)\, e^{i\phi_\theta(\sigma)}, \qquad \psi_\theta(\sigma) > 0, \tag{64}$$

where $\psi_\theta$ and $\phi_\theta$ denote the learnable amplitudes and phases. The variational Monte Carlo estimator for the energy is

$$E(\theta) = \sum_\sigma \Pi_\theta(\sigma)\, E_{\mathrm{loc}}(\sigma;\theta), \qquad \Pi_\theta(\sigma) = \frac{|\Psi_\theta(\sigma)|^2}{\sum_{\sigma'} |\Psi_\theta(\sigma')|^2}. \tag{65}$$

For the $J_1 - J_2$ Hamiltonian with off-diagonal matrix elements $H^{\pm}_{\sigma\sigma'}$, the phase-sensitive contribution to the energy is

$$E_\phi(\theta) = \sum_\sigma \Pi_\theta(\sigma) \sum_{\sigma'} H^{\pm}_{\sigma\sigma'}\, \frac{\psi_\theta(\sigma')}{\psi_\theta(\sigma)} \cos\big[\phi_\theta(\sigma) - \phi_\theta(\sigma')\big]. \tag{66}$$

To expose the implicit discrete structure, we isolate the amplitudes and define

$$\rho_{\sigma\sigma'}(\theta) = \frac{\psi_\theta(\sigma')}{\psi_\theta(\sigma)}. \tag{67}$$

Restricting phases to the $Z_2$ manifold,

$$\phi_\theta(\sigma) \in \{0, \pi\} \qquad \Rightarrow \qquad \cos\big[\phi_\theta(\sigma) - \phi_\theta(\sigma')\big] = s_\sigma s_{\sigma'}, \qquad s_\sigma \in \{\pm 1\}, \tag{68}$$

Eq. (66) becomes a quadratic form in the sign variables,

$$E_\phi[s] = \sum_\sigma \Pi_\theta(\sigma) \sum_{\sigma'} H^{\pm}_{\sigma\sigma'}\, \rho_{\sigma\sigma'}(\theta)\, s_\sigma s_{\sigma'}. \tag{69}$$

For the $J_1$–$J_2$ model, the off-diagonal elements naturally split as

$$H^{\pm}_{\sigma\sigma'} = J_1 K^{(1)}_{\sigma\sigma'} + J_2 K^{(2)}_{\sigma\sigma'}, \tag{70}$$

where $K^{(1)}_{\sigma\sigma'}$ ($K^{(2)}_{\sigma\sigma'}$) is nonzero only when $\sigma$ and $\sigma'$ differ by a single nearest-neighbour (next-nearest-neighbour) spin flip. Define

$$C^{(a)}_{\sigma\sigma'} := \Pi_\theta(\sigma)\, K^{(a)}_{\sigma\sigma'}\, \rho_{\sigma\sigma'}(\theta), \qquad a = 1, 2, \tag{71}$$

and symmetrise to obtain a real symmetric interaction,

$$J^{(a)}_{\sigma\sigma'} = \frac{1}{2}\left(C^{(a)}_{\sigma\sigma'} + C^{(a)}_{\sigma'\sigma}\right). \tag{72}$$

Insertion into Eq. (69) gives

$$E_\phi[s] = J_1 \sum_{\sigma<\sigma'} J^{(1)}_{\sigma\sigma'} s_\sigma s_{\sigma'} + J_2 \sum_{\sigma<\sigma'} J^{(2)}_{\sigma\sigma'} s_\sigma s_{\sigma'}. \tag{73}$$

Introduce the effective interaction

$$\widetilde{J}_{\sigma\sigma'}(\theta; J_1, J_2) = J_1 J^{(1)}_{\sigma\sigma'}(\theta) + J_2 J^{(2)}_{\sigma\sigma'}(\theta), \tag{74}$$

which combines all edges of the configuration graph connected by a single NN or NNN spin flip. Then the phase sector becomes

$$E_\phi[s] = \sum_{\sigma<\sigma'} \widetilde{J}_{\sigma\sigma'}(\theta; J_1, J_2)\; s_\sigma s_{\sigma'}. \tag{75}$$

Equation (75) is exactly a quadratic unconstrained binary optimization (QUBO) or, equivalently, the Ising spin-glass ground-state problem on the configuration graph.

## DIRICHLET ENERGY AND GRAPH LAPLACIAN

We begin from Eq. (13), which gives the phase–dependent contribution to the variational energy once the amplitudes $\{\psi_\sigma\}$ are fixed,

$$E_q = \frac{1}{Z} \sum_{\{\sigma,\tau\}\in\mathcal{E}} W^{\Gamma}_{\sigma\tau}(J_1, J_2)\; \cos\bigl(\phi_\sigma - \phi_\tau\bigr). \tag{76}$$

Here $\mathcal{E}$ denotes the set of undirected edges of the configuration graph $\Gamma(G)$, and

$$W^{\Gamma}_{\sigma\tau}(J_1, J_2) := \sum_{r=1}^{2} J_r\, W^{(r)}_{\sigma\tau},$$

which vanishes unless $\{\sigma, \tau\} \in \mathcal{N}_1 \cup \mathcal{N}_2$. Once the amplitudes are fixed, the weights $W^{\Gamma}_{\sigma\tau}$ are fixed as well. Using the identity

$$\cos(\phi_\sigma - \phi_\tau) = 1 - \frac{1}{2}\bigl|e^{i\phi_\sigma} - e^{i\phi_\tau}\bigr|^2,$$

and identifying

$$e^{i\phi_\sigma} \;\longleftrightarrow\; u_\sigma := (\cos\phi_\sigma, \sin\phi_\sigma)^\top \in \mathbb{R}^2,$$

we may write

$$\cos(\phi_\sigma - \phi_\tau) = 1 - \frac{1}{2}\, \|u_\sigma - u_\tau\|^2. \tag{77}$$

Substituting Eq. (77) into Eq. (76) yields

$$E_q = \frac{1}{Z} \sum_{r=1}^{2} J_r \sum_{\{\sigma,\tau\}\in\mathcal{N}_r} W^{(r)}_{\sigma\tau} \left[1 - \frac{1}{2}\|u_\sigma - u_\tau\|^2\right]. \tag{78}$$

This naturally splits into a constant term and a phase–dependent term,

$$E_q = E_0 - E_\phi,$$

with

$$E_0 = \frac{1}{Z} \sum_{r=1}^{2} J_r \sum_{\{\sigma,\tau\}\in\mathcal{N}_r} W^{(r)}_{\sigma\tau}, \tag{79}$$

$$E_\phi = \frac{1}{2Z} \sum_{r=1}^{2} J_r \sum_{\{\sigma,\tau\}\in\mathcal{N}_r} W^{(r)}_{\sigma\tau}\; \|u_\sigma - u_\tau\|^2. \tag{80}$$

The quantity $E_\phi$ is a weighted *Dirichlet energy* for the phase field on the configuration graph.

To express this in matrix form, collect the phase vectors into

$$U := [\,c \;\; s\,] \in \mathbb{R}^{n\times 2}, \qquad c_\sigma = \cos\phi_\sigma, \;\; s_\sigma = \sin\phi_\sigma.$$

Noting that

$$\|u_\sigma - u_\tau\|^2 = u_\sigma^\top u_\sigma + u_\tau^\top u_\tau - 2\, u_\sigma^\top u_\tau, \tag{81}$$

and using the symmetry of the undirected graph, one finds

$$E_\phi = \frac{1}{2Z}\sum_{r=1}^{2} J_r \left[\sum_\sigma d_\sigma^{(r)}\, u_\sigma^\top u_\sigma - \sum_{\sigma,\tau} W_{\sigma\tau}^{(r)}\, u_\sigma^\top u_\tau\right], \tag{82}$$

where

$$d_\sigma^{(r)} := \sum_\tau W_{\sigma\tau}^{(r)}$$

is the weighted degree.

Introducing the weighted adjacency matrix

$$W^{(r)} := \big(W_{\sigma\tau}^{(r)}\big)_{\sigma,\tau=1}^{n},$$

the degree matrix

$$D^{(r)} := \mathrm{Diag}\big(d_1^{(r)}, \ldots, d_n^{(r)}\big),$$

and the graph Laplacian

$$L^{(r)} := D^{(r)} - W^{(r)},$$

the Dirichlet energy takes the compact form

$$E_\phi = \frac{1}{2Z}\sum_{r=1}^{2} J_r \,\mathrm{Tr}\Big(U^\top L^{(r)} U\Big). \tag{83}$$

Minimization of $E_\phi$ is subject to the unit–norm constraints $\|u_\sigma\|^2 = 1$ for all $\sigma$. Introducing Lagrange multipliers $\lambda_\sigma$ and varying

$$\mathcal{F}[U,\lambda] = E_\phi - \frac{1}{2}\sum_\sigma \lambda_\sigma \left(u_\sigma^\top u_\sigma - 1\right), \tag{84}$$

we obtain the stationarity condition

$$\frac{1}{Z}\left(\sum_{r=1}^{2} J_r L^{(r)} U\right)_\sigma = \lambda_\sigma\, u_\sigma, \qquad \forall\,\sigma. \tag{85}$$

This is a *local* eigenvalue condition, with $\lambda_\sigma$ enforcing the unit–length constraint at each vertex.

Projecting Eq. (85) onto the direction orthogonal to $u_\sigma$ yields the explicit phase–balance equations

$$\sum_{r=1}^{2} J_r \sum_{\tau\in\mathcal{N}_r(\sigma)} W_{\sigma\tau}^{(r)}\, \sin(\phi_\sigma - \phi_\tau) = 0, \qquad \forall\,\sigma. \tag{86}$$

These nonlinear KKT [9, 10] equations fully determine the optimal phase configuration on the c-graph.

## PHASE OPTIMIZATION FOR $2 \times 2$ SQUARE LATTICE HAF

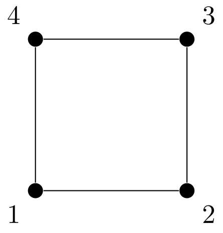


Total $S_z = 0$, states are

$$|\sigma_1\rangle = |\uparrow_1\uparrow_2\downarrow_3\downarrow_4\rangle\,, \qquad |\sigma_2\rangle = |\downarrow_1\downarrow_2\uparrow_3\uparrow_4\rangle \tag{87}$$

$$|\sigma_3\rangle = |\uparrow_1\downarrow_2\uparrow_3\downarrow_4\rangle\,, \qquad |\sigma_4\rangle = |\downarrow_1\uparrow_2\downarrow_3\uparrow_4\rangle \tag{88}$$

$$|\sigma_5\rangle = |\uparrow_1\downarrow_2\downarrow_3\uparrow_4\rangle\,, \qquad |\sigma_6\rangle = |\downarrow_1\uparrow_2\uparrow_3\downarrow_4\rangle \tag{89}$$

For a bond $(i,j)$, the spin-flip part is $\hat{H}^{\pm}_{ij} = \hat{S}^+_i\hat{S}^-_j + \hat{S}^-_i\hat{S}^+_j$. and it only acts when spins at $i,j$ are antiparallel; otherwise, it gives zero. Each nonzero action connects two configurations by a single NN swap. $\tau \in \mathcal{N}_1(\sigma)$ (reachable by one NN flip) and $\tau \in \mathcal{N}_2(\sigma)$ (reachable by one NNN flip).

| State $\sigma$ | $\mathcal{N}_1(\sigma)$ (NN flips) | $\mathcal{N}_2(\sigma)$ (NNN flips) |
|---|---|---|
| $\sigma_1$ | $\{\sigma_3,\,\sigma_4\}$ | $\{\sigma_5,\,\sigma_6\}$ |
| $\sigma_2$ | $\{\sigma_3,\,\sigma_4\}$ | $\{\sigma_5,\,\sigma_6\}$ |
| $\sigma_3$ | $\{\sigma_1,\,\sigma_2\}$ | $\{\sigma_5,\,\sigma_6\}$ |
| $\sigma_4$ | $\{\sigma_1,\,\sigma_2\}$ | $\{\sigma_5,\,\sigma_6\}$ |
| $\sigma_5$ | $\{\sigma_6\}$ | $\{\sigma_1,\,\sigma_2,\,\sigma_3,\,\sigma_4\}$ |
| $\sigma_6$ | $\{\sigma_5\}$ | $\{\sigma_1,\,\sigma_2,\,\sigma_3,\,\sigma_4\}$ |

TABLE I: Neighbour sets $\mathcal{N}_1$ and $\mathcal{N}_2$ for the $L = 4$ c-graph under the J$_1$–J$_2$ Heisenberg off-diagonal dynamics.

$$E_{nn}/2J_1 = \psi_1\psi_3\cos(\phi_1-\phi_3) + \psi_1\psi_4\cos(\phi_1-\phi_4) + \psi_2\psi_3\cos(\phi_2-\phi_3) + \psi_2\psi_4\cos(\phi_2-\phi_4) \tag{90}$$
$$+\,\psi_5\psi_3\cos(\phi_5-\phi_3) + \psi_6\psi_3\cos(\phi_6-\phi_3) + \psi_6\psi_4\cos(\phi_6-\phi_4) + \psi_4\psi_5\cos(\phi_5-\phi_4) \tag{91}$$

Taking the derivatives with respect to phases gives

$$\psi_1\psi_3\sin(\phi_1-\phi_3) + \psi_1\psi_4\sin(\phi_1-\phi_4) = 0 \tag{92}$$
$$\psi_2\psi_3\sin(\phi_2-\phi_3) + \psi_2\psi_4\sin(\phi_2-\phi_4) = 0 \tag{93}$$
$$\psi_5\psi_3\sin(\phi_5-\phi_3) + \psi_5\psi_4\sin(\phi_5-\phi_4) = 0 \tag{94}$$
$$\psi_6\psi_3\sin(\phi_6-\phi_3) + \psi_6\psi_4\sin(\phi_6-\phi_4) = 0 \tag{95}$$

Lets take derivative wrt $\phi_3$ and $\phi_4$

$$\psi_1\psi_3\sin(\phi_1-\phi_3) + \psi_2\psi_3\sin(\phi_2-\phi_3) + \psi_3\psi_5\sin(\phi_5-\phi_3) + \psi_3\psi_6\sin(\phi_6-\phi_3) = 0 \tag{96}$$
$$\psi_1\psi_4\sin(\phi_1-\phi_4) + \psi_2\psi_4\sin(\phi_2-\phi_4) + \psi_4\psi_5\sin(\phi_5-\phi_4) + \psi_4\psi_6\sin(\phi_6-\phi_4) = 0 \tag{97}$$

Because the energy depends only on phase *differences*, the KKT system is invariant under a global shift $\phi_\sigma \longrightarrow \phi_\sigma + \alpha$. This one–parameter gauge redundancy may be removed by fixing a single phase. We choose $\phi_3 = 0$. Because the phase is only defined on configurations with nonzero amplitude, the KKT equations are imposed only on vertices with $\psi_\sigma > 0$; vertices with $\psi_\sigma = 0$ drop out automatically since their derivative conditions are identically satisfied. Therefore

$$\psi_3\sin(\phi_1-\phi_3) + \psi_4\sin(\phi_1-\phi_4) = 0 \tag{98}$$
$$\psi_3\sin(\phi_2-\phi_3) + \psi_4\sin(\phi_2-\phi_4) = 0 \tag{99}$$
$$\psi_3\sin\phi_5 + \psi_4\sin(\phi_5-\phi_4) = 0 \tag{100}$$
$$\psi_3\sin\phi_6 + \psi_4\sin(\phi_6-\phi_4) = 0 \tag{101}$$

$$\psi_1 \sin\phi_1 + \psi_2 \sin(\phi_2 - \phi_3) + \psi_5 \sin(\phi_5 - \phi_3) + \psi_6 \sin(\phi_6 - \phi_3) = 0 \tag{102}$$

$$\psi_1 \sin(\phi_1 - \phi_4) + \psi_2 \sin(\phi_2 - \phi_4) + \psi_5 \sin(\phi_5 - \phi_4) + \psi_6 \sin(\phi_6 - \phi_4) = 0 \tag{103}$$

Solving them gives

$$\tan\phi_1 = \tan\phi_2 = \tan\phi_5 = \tan\phi_6 = \frac{\psi_4 \sin\phi_4}{(\psi_3 + \psi_4 \cos\phi_4)} \tag{104}$$

Therefore

$$\phi_1 = \phi_2 = \phi_5 = \phi_6 := \gamma \tag{105}$$

Then

$$(\psi_1 + \psi_2 + \psi_5 + \psi_6) \sin\gamma = 0 \tag{106}$$

Therefore

$$\gamma \in \{0, \pi\} \tag{107}$$

Inserting it into second equation we get

$$(\psi_1 + \psi_2 + \psi_5 + \psi_6) \sin(\gamma - \phi_4) = 0 \tag{108}$$

Therefore

$$\phi_4 \in \{\gamma, \gamma + \pi\} \tag{109}$$

Let's now find out the solution for the global minima:

- $\gamma = 0$, $\phi_4 = 0$, all terms in the $E_{nn}$ is positive. Therefore, it does not correspond to global minima (in fact, the energy becomes max!).
- $\gamma = \pi$, $\phi_4 = \pi$, bonds has mixed sign. Therefore, it does not correspond to a global minimum.
- $\gamma = 0$, $\phi_4 = \pi$, bonds has mixed sign. Therefore, it does not correspond to global minima.
- $\gamma = \pi$, $\phi_4 = 0$, the energy become:

$$E_{nn}/2J_1 = \psi_1\psi_3 \cos(\phi_1) + \psi_1\psi_4 \cos(\phi_1) + \psi_2\psi_3 \cos(\phi_2) + \psi_2\psi_4 \cos(\phi_2) \tag{110}$$

$$+ \psi_5\psi_3 \cos(\phi_5) + \psi_6\psi_3 \cos(\phi_6) + \psi_6\psi_4 \cos(\phi_6) + \psi_4\psi_5 \cos(\phi_5) \tag{111}$$

$$E_{nn} = -2J_1 \Big(\psi_1\psi_3 + \psi_1\psi_4 + \psi_2\psi_3 + \psi_2\psi_4 + \psi_5\psi_3 + \psi_6\psi_3 + \psi_6\psi_4 + \psi_4\psi_5\Big) \tag{112}$$

This is the lowest-energy configuration of the system. Thus, the two equivalent AFM minima are:

$$(\phi_1, \phi_2, \phi_3, \phi_4, \phi_5, \phi_6) = (\pi, \pi, \pi, \pi, 0, 0) \quad \text{or} \quad (0, 0, 0, 0, \pi, \pi) \tag{113}$$


[1] W. Marshall, Proceedings of the Royal Society of London. Series A. Mathematical and Physical Sciences **232**, 48 (1955).
[2] S. Rao, *Field Theories in Condensed Matter Physics* (CRC Press, 2019).
[3] P. Fazekas, *Lecture Notes on Electron Correlation and Magnetism* (1999).
[4] R. Fabila-Monroy, D. Flores-Peñaloza, C. Huemer, F. Hurtado, J. Urrutia, and D. R. Wood, Graphs and Combinatorics **28**, 365 (2012).
[5] T. Westerhout, M. I. Katsnelson, and A. A. Bagrov, Commun. Phys. **6**, 275 (2023), arXiv:2207.10675 [cond-mat.dis-nn].
[6] E. Lieb and D. Mattis, Journal of Mathematical Physics **3**, 749 (1962).
[7] M. X. Goemans and D. P. Williamson, Journal of the ACM (JACM) **42**, 1115 (1995).
[8] S. Boyd and L. Vandenberghe, *Convex Optimization* (Cambridge University Press, 2004).
[9] W. Karush, *Minima of functions of several variables with inequalities as side conditions*, Master's thesis, Department of Mathematics, University of Chicago, Chicago, Illinois (1939).
[10] H. W. Kuhn and A. W. Tucker, in *Proceedings of the Second Berkeley Symposium on Mathematical Statistics and Probability* (University of California Press, 1951) pp. 481–492.
